# Supplementary material for: Self-induced polar order of active Brownian particles in a harmonic trap
Source: arXiv:1402.1397 source file (2014-02-06)
Supplement: Supplementary file 1 [file Supplemental_final.pdf]

# Supplemental material

Marc Hennes, Katrin Wolff, and Holger Stark
*Institut für Theoretische Physik, Technische Universität Berlin, Hardenbergstraße 36, 10623 Berlin, Germany*
(Dated: February 6, 2014)

## SIMULATION METHOD

Brownian dynamics simulations with hydodynamic interactions were performed using the algorithm by Ermak and McCammon [1] adapted for active particles. Positions for $N$ particles are updated via a simple Euler scheme

$$\mathbf{r}_i(t+\Delta t) = \mathbf{r}_i(t) + \left( v_0\mathbf{p}_i + \sum_{j=1}^{N} \boldsymbol{\mu}_{ij}^{tt}\mathbf{F}_j + \sum_{j\neq i}^{N} \mathbf{u}_{\mathrm{SS}}(\mathbf{r}_{ij}) \right) \Delta t + \sum_{j=1}^{2N} \mathbf{H}_{ij}\boldsymbol{\xi}_j \sqrt{\Delta t}. \quad (1)$$

where $v_0\mathbf{p}_i$ and $\mathbf{u}_{\mathrm{SS}}(\mathbf{r}_{ij})$ are contributions due to the particles' activity. The particle's intrinsic swimming speed is $v_0$, its instantaneous orientation $\mathbf{p}_i$, and $\mathbf{u}_{\mathrm{SS}}(\mathbf{r}_{ij})$ is the stresslet generated by each swimmer

$$\mathbf{u}_{\mathrm{SS}}(\mathbf{r}_{ij}) = \frac{3\beta v_0}{4\pi r_{ij}^2}\left(-3(\mathbf{p}_j\cdot\hat{\mathbf{r}}_{ij})^2 + 1\right)\hat{\mathbf{r}}_{ij}, \quad (2)$$

where $\mathbf{r}_{ij}$ is the vector connecting particles $i$ and $j$ and $\hat{\mathbf{r}}_{ij} = \mathbf{r}_{ij}/r_{ij}$. The parameter $\beta$ determines whether a particle is extensile (pusher, $\beta < 0$), contractile (puller, $\beta > 0$ or neutral $\beta = 0$ [2]. If not stated otherwise, we use the neutral swimmer so $\mathbf{u}_{\mathrm{SS}}(\mathbf{r}_{ij}) = 0$. Furthermore, each particle feels the harmonic trapping force $\mathbf{F}_j = -k_{\mathrm{trap}}\mathbf{r}_j$ and hydroynamic interactions between the particles are described by the translational mobility tensor $\boldsymbol{\mu}_{ij}^{tt}$ on the Oseen level. The thermal noise term $\sum_{j=1}^{2N}\mathbf{H}_{ij}\boldsymbol{\xi}_j$ also couples particles to each other, where each of the $2N$ vectors $\boldsymbol{\xi}_i$ for translational and rotational noise contains three independent, Gaussian distributed random numbers with unit variance. At the end of each position update, volume exclusion is implemented by checking and correcting the interparticle distance to the particle diameter if $r_{ij} < 2a$.

Similarly to the positions in Eq. (1), the orientations are updated according to

$$\mathbf{p}_i(t+\Delta t) = \mathbf{p}_i(t) + \left(\boldsymbol{\omega}_{\mathrm{det},i}\times\mathbf{p}_i(t) - 2\mu_r k_B T\mathbf{p}_i\right)\Delta t + \left(\sum_{j=1}^{2N}\mathbf{H}_{(i+N)j}\boldsymbol{\xi}_j \times \mathbf{p}_i\right)\sqrt{\Delta t} \quad (3)$$

where $\boldsymbol{\omega}_{\mathrm{det},i}$ denotes the deterministic angular velocity of each particle $i$, given by

$$\boldsymbol{\omega}_{\mathrm{det},i}(\mathbf{r}_i) = \sum_{j=1}^{N}\boldsymbol{\mu}_{ij}^{tr}\mathbf{F}_j + \sum_{j\neq i}^{N}\frac{1}{2}\left[\nabla_{\mathbf{r}_i}\times\mathbf{u}_{\mathrm{SS}}(\mathbf{r}_{ij})\right]. \quad (4)$$

The additional term $-2\mu_r k_B T\mathbf{p}_i\Delta t$ in Eq. (3) arises because the Langevin equation is interpreted in the Stratonovich sense and has to be recast into the Itō form for simulations within the Euler forward scheme. The thermal noise contribution $\sum_{j=1}^{2N}\mathbf{H}_{(i+N)j}\boldsymbol{\xi}_j$ again couples translational and rotational stochastic motion of all particles. The matrix $\mathbf{H}$ is connected to the grand mobility matrix $\mathbf{M}$ through the Einstein relation

$$\mathbf{H}\mathbf{H}^T = 2k_B T\mathbf{M}, \quad (5)$$

and, in the absence of hydrodynamic coupling, reduces to $\sqrt{2D}$ for translational and $\sqrt{2D_R}$ for rotational motion. The grand mobility matrix $\mathbf{M}$ in turn consists of the individual mobility tensors $\boldsymbol{\mu}_{ij}$ for translation and rotation $\mathbf{M} = \begin{pmatrix}\boldsymbol{\mu}_{ij}^{tt} & \boldsymbol{\mu}_{ij}^{tr}\\ \boldsymbol{\mu}_{ij}^{rt} & \boldsymbol{\mu}_{ij}^{rr}\end{pmatrix}$ which, to order $\mathcal{O}(r_{ij}^{-2})$ in inverse particle distances $r_{ij}$, are

$$\begin{aligned}
\boldsymbol{\mu}_{ii}^{tt} &= \mu_t\mathbf{1}\\
\boldsymbol{\mu}_{ij}^{tt} &= \frac{3\mu_t}{4}\frac{a}{r_{ij}}(\mathbf{1} + \hat{\mathbf{r}}_{ij}\otimes\hat{\mathbf{r}}_{ij})\\
\boldsymbol{\mu}_{ii}^{rr} &= \mu_r\mathbf{1}\\
\boldsymbol{\mu}_{ij}^{rr} &= 0\\
\boldsymbol{\mu}_{ii}^{tr} &= \boldsymbol{\mu}_{ii}^{rt} = 0\\
\boldsymbol{\mu}_{ij}^{tr} &= \boldsymbol{\mu}_{ij}^{rt} = \mu_r a\left(\frac{a}{r_{ij}}\right)^2\hat{\mathbf{r}}_{ij}\times.
\end{aligned} \quad (6)$$

Here, $\mathbf{1}$ stands for the $3\times3$ unit matrix, $a$ for the swimmer radius and $\mu_t = 1/(6\pi\eta a)$, $\mu_r = 1/(8\pi\eta a^3)$ denote the Stokes mobility coefficients for the translation and rotation of a sphere. Note that for this form of $\mathbf{M}$ the spurious drift term proportional to the divergence of $\mathbf{M}$ vanishes.

## PUMP FORMATION – COMPARISON OF TIME SCALES

In the non-interacting system at high enough activity Pe, active particles accumuluate at the surface of a sphere with radius $r_{\mathrm{hor}} = a\mathrm{Pe}/\alpha = v_0 6\pi\eta a/k_{\mathrm{trap}}$ with their velocity vectors pointing outward such that self-propulsion and trapping force cancel. Here the active Péclet number is $\mathrm{Pe} = v_0 a/D$ and the trapping Péclet number is $\alpha = k_{\mathrm{trap}}a^2/(k_{\mathrm{B}}T)$ with the thermal diffusion coefficient $D = k_{\mathrm{B}}T/(6\pi\eta a)$. In our Brownian dynamics simulations we observe that, irrespective of initial conditions, particles first swim predominantly towards these

steady-state positions of the non-interacting system before pump formation starts (see also the two movies in the supplemental material). We can thus base the criterion for pump formation on a comparison of time scales in this spherically symmetric state. Specifically, we compare the time it takes a particle to rotate by diffusion $T_{\rm diff} = 2\pi^2/D_R$ with the time for rotation by the flow field's vorticity $T_{\rm HI} = 2\pi/\omega_{\rm HI}$. Here, the thermal rotational diffusion coefficient is $D_R = 3D/(4a^2)$.

To this end we assume that the flow fields due to all particles approximately cancel each other except for a single excess particle $j$, which creates a flow field at the position of its nearest-neighbor particle $i$,

$$\mathbf{u}_i = \frac{1}{8\pi\eta r_{ij}} \left(\mathbf{1} + \hat{\mathbf{r}}_{ij} \otimes \hat{\mathbf{r}}_{ij}\right) \mathbf{F}_j. \tag{7}$$

The corresponding vorticity is

$$\boldsymbol{\omega}_{{\rm HI},i} = \frac{1}{8\pi\eta r_{ij}^2} \hat{\mathbf{r}}_{ij} \times \mathbf{F}_j. \tag{8}$$

With particles accumulated at $r_{\rm hor}$ and $\hat{\mathbf{r}}_{ij}$ approximately perpendicular to $\mathbf{F}_j$, we thus find $\omega_{{\rm HI},i} = k_{\rm trap} r_{\rm hor}/(8\pi\eta r_{ij}^2)$. A characteristic quantity for the distance between neighboring particles follows from $4\pi r_{\rm hor} \approx N\pi(r_{ij}/2)^2$ and gives $r_{ij} \approx 4r_{\rm hor}/\sqrt{N}$. The requirement for pump formation, i.e. that particle $i$ rotates with its swimming direction towards particle $j$ and thereby enhances the density excess, is $T_{\rm diff} > T_{\rm HI}$. Then, with the above definition of $r_{\rm hor}$ the criterion for pump formation follows,

$$\alpha > 4\sqrt{{\rm Pe}/(\pi N)}. \tag{9}$$

## MEAN FIELD THEORY

In order to make analytical predictions, we reduce the many-particle system to a mean field system, where a single particle experiences a mean flow field $\mathbf{u}(\mathbf{r})$ set up by all the particles. The joint positional and orientational distribution function $\psi(\mathbf{r}, \mathbf{p})$ follows from the Smoluchowski equation

$$\partial_t \psi(\mathbf{r}, \mathbf{p}) = -\nabla \cdot \mathbf{J}_T - \mathcal{R} \cdot \mathbf{J}_R \quad \text{where} \quad \mathcal{R} = \mathbf{p} \times \nabla_{\mathbf{p}} \tag{10}$$

where $\mathbf{J}_T = [v_0\mathbf{p} + \mu_t \mathbf{F}_{\rm ext}(\mathbf{r}) + \mathbf{u}(\mathbf{r})]\psi(\mathbf{r}, \mathbf{p})$ is the translational flux and $\mathbf{J}_R = [(\nabla \times \mathbf{u}(\mathbf{r}))/2 - D_R\mathcal{R}]\psi(\mathbf{r}, \mathbf{p})$ the rotational flux. Translational diffusion has been neglected in $\mathbf{J}_T$ because of Péclet numbers ${\rm Pe} \gtrsim 100$, whereas in the rotational case diffusion is still non-negligible.

In our Brownian dynamics simulations we observed that the collective flow field in the steady-state closely follows a regularized stokeslet (see main text)

$$\mathbf{u}_{\rm reg}(\mathbf{r}) = -\frac{v_0\epsilon}{(r^2 + 2\epsilon^2)^{3/2}} [\mathbf{1}(r^2 + 2\epsilon^2) + \mathbf{r} \otimes \mathbf{r}]\mathbf{e}_z, \tag{11}$$

where $\epsilon$ is a fitting parameter which matches the pump radius for the region actually populated by particles. Eq. (11) and thus Eq. (10) only describe the dynamics close to a fully formed pump state and we will only attempt to determine the steady state distribution $\psi(\mathbf{r}, \mathbf{p})$.

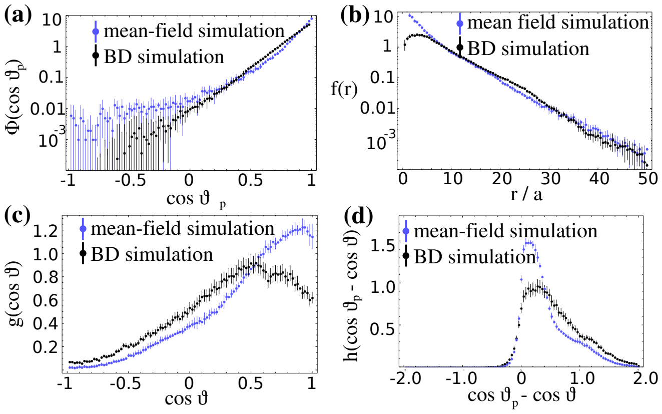


FIG. 1. (Color online.) Comparison of mean field and Brownian dynamics simulations for **(a)** orientational distribution function $\Phi(\cos\theta_p)$, **(b)** radial positional distribution $f(r)$, **(c)** angular positional distribution $g(\cos\theta)$ and **(d)** the distribution function for the difference in orientational and positional polar angle $h(\cos\theta_p - \cos\theta)$.

We first demonstrate how well the mean field theory works. Fig. 1 compares simulation results of Eq. (10) using Eq. (11) with results of the full $N$-particle Brownian dynamics simulations for ${\rm Pe} = 500$ and shows good agreement. The orientational distribution functions $\Phi(\cos\theta_p)$ in Fig. 1 **(a)** agree very well. Note that in Fig. 3 of the main text Brownian dynamics simulations are plotted together with the analytical approximation of Eq. (10). The radial position distribution function $f(r) = \int \psi(\mathbf{r}, \mathbf{p}) d^2\mathbf{p} d\Omega_r$ is shown in Fig. 1 **(b)** with very good agreement except at very small distances meaning close to the centre of the trap. Fig. 1 **(c)** plots the distribution functions $g(\cos\theta)$ for the polar angle $\theta$ of the position vector. Here, mean field simulations over-estimate the occurrence of large $\cos\theta$, that is the focussing of the pump. We presume that both this effect and the discrepancy in $f(r)$ at small $r$ are due to excluded volume effects in the $N$ particle simulations. Fig. 1 **(d)** finally shows the distribution functions for the difference between orientation and position angles $\Delta = \cos\theta_p - \cos\theta$. As both angles $\theta_p$ and $\theta$ are measured against the pump main axis, $h(\Delta)$ indicates how well a particle's position and orientation vector are aligned and how well the assumption $\psi(\mathbf{r}, \mathbf{p}) = \Phi(\mathbf{p})\, f(r)\, \delta(\cos\theta - \cos\theta_p)\delta(\varphi - \varphi_p)$ used to approximately solve Eq. (10) holds.

With above ansatz for $\psi(\mathbf{r}, \mathbf{p})$ we find $\Phi(\mathbf{p}) = \exp(A\cos\theta_p)/\mathcal{N}$ with $A = {\rm Pe} \int_0^\infty \frac{\epsilon\, a(5\epsilon^2 + 2r^2)}{3(\epsilon^2 + r^2)^{5/2}} r^3 f(r) {\rm d}r$ (see main text). The parameter $A$ thus plays the role of Weiss' molecular field and aligns particle directions $\mathbf{p}$

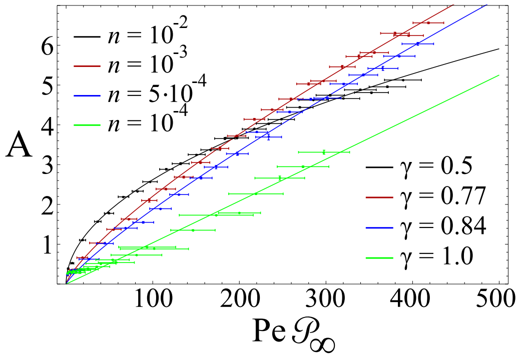


FIG. 2. (Color online.) Field strength $A$ over $\mathcal{P}_\infty$Pe for different densities $n$. The solid lines are fits to $A \propto (\mathcal{P}_\infty \mathrm{Pe})^\gamma$ with the exponent $\gamma$ given in the graph.

along a common axis. The field $A$ in turn depends on particle alignment $\mathcal{P}_\infty$ and Pe. To show this, we plot $A$ over Pe$\mathcal{P}_\infty$ for different densities $n$ in Fig. 2 and find a scaling according to $A \propto (\mathrm{Pe}\mathcal{P}_\infty)^\gamma$. For low densities, we find a linear increase ($\gamma = 1$) as in the classical mean field theory of ferromagnetism and with growing densities the increase becomes sublinear ($\gamma < 1$).


[1] D. L. Ermak and J. A. McCammon, J. Chem. Phys. **69**, 1352 (1978).

[2] T. Ishikawa, M. P. Simmonds, and T. J. Pedley, J. Fluid Mech. **568**, 119 (2006).
